# Supplementary material for: An algebraic multigrid method for $Q_2-Q_1$ mixed discretizations of the Navier-Stokes equations
Source: arXiv:1607.02489 source file (2017-03-07)
Supplement: Supplementary file 1 [file appendix.tex]

\subsection{Algorithm to construct $\tilde{A}^{(p)}$ and $\tilde{A}^{(v)}$}\label{s:appendix_dropping}
Algorithm~\ref{a:filtering} demonstrates the filtering procedure for a given
matrix. The goal of the filtering is to compact the stencil of a matrix produced
using quadratic basis functions as such matrices have a wider stencil compared
to those obtained with first order functions.

\begin{algorithm}[h!]
\caption{$[\tilde{A}^{(v)},\tilde{A}^{(p)}] = \mbox{\func{form\_aux\_block\_diagonal}}(\mathcal{A}, tol)$}
\label{a:filtering}
\begin{algorithmic}
  \State Assuming $\mathcal{A} = \begin{pmatrix} A & B^T \\ B & 0 \end{pmatrix}$ \\[    ]

  \State $Z = A,\; Z = \{z_{ij}\}$
  \State $(\tilde{A}^{(v)})_{ij} = \begin{cases}
    0,       & \mbox{if}\quad |z_{ij}| \le tol \, \sqrt{z_{ii} z_{jj}}, \\
    z_{ij},  & \mbox{otherwise}.
  \end{cases}$
  \State $(\tilde{A}^{(v)})_{ii} = (\tilde{A}^{(v)})_{ii} - \left(\tilde{A}^{(v)} {\bf e}\right)_i$ \\[    ]

  \State $Z = BB^T,\; Z = \{z_{ij}\}$
  \State $(\tilde{A}^{(p)})_{ij} = \begin{cases}
    0,       & \mbox{if}\quad |z_{ij}| \le tol \, \sqrt{z_{ii} z_{jj}}, \\
    z_{ij},  & \mbox{otherwise}.
  \end{cases}$
  \State $(\tilde{A}^{(p)})_{ii} = (\tilde{A}^{(p)})_{ii} - \left(\tilde{A}^{(p)} {\bf e}\right)_i$

\end{algorithmic}
\end{algorithm}
\unsure{AP}{Actually, in MueLu we use no lumping, but it produces same results
as lumping in Matlab. Why?}

\subsection{Algorithm to update heuristics}\label{s:appendix_heuristics}
Algorithm~\ref{a:update_heuristics} demonstrates the update procedure for the
set of heuristics $h_1$ and $h_2$ that are used in computations to
a) encourage close packing of coarse points, and b) convert additional $F$-points
that are not well covered by $C$-points to $C$-points. Both heuristics are
updated each time a new $C$-point is selected. The initial values of $h_1$ are
set to $10^4$ times the diameter of the set of coordinates, and initial values
of $h_2$ are set to zero.

\begin{algorithm}[h!]
\caption{$[h_1, h_2] = \mbox{\func{update\_heuristics}}(V, E, S, x, k, h_1, h_2)$}
\label{a:update_heuristics}
  \begin{algorithmic}
    \State $D_4 = \{ ~j ~|~ dist(V_k,V_j, E) \le 4~ \}$ \\[    ]

    \For{$j \in D_4$}
      \State $h_1(j) = \dfrac{2 h_1(j) \|x_j - x_k\|}{h_1(j) + \|x_j - x_k\|}$
      \State $h_2(j) = \left(h_2(j)(|S_j|-1) + dist(V_k, V_j, E)\right)/|S_j|$
    \EndFor

  \end{algorithmic}
\end{algorithm}

The vertices in the $Cand$ set are sorted by their $h_1$ values, and the next
chosen vertex has the smallest value.

\subsection{Algorithm to add extra $C$-points}\label{s:appendix_extra_dist3_Cpoints}
This function finds $F$-points not well covered by the current set of
$C$-points, and converts some of these to $C$-points. The internal parameters
are chosen to be $\omega_g = 0.8$ and $\omega_o = 0.5$.

\begin{algorithm}[h!]
\caption{$[C, F, S] = \mbox{\func{find\_extra\_dist3\_Cpoints}}(V, E, S, C, F, x, h_1, h_2)$}
  \begin{algorithmic}
    \For{$t = 1, 2$}
      \State $Cand = \{~j ~|~ |S_j| = t~\}$

      \State $h_1^{max} = \max_{j \in Cand} h_1(j)$
      \State $h_2^{max} = \max_{j \in Cand} h_2(j)$

      \State $h(j) = -(\omega_g h_2(j)/h_2^{max} + (1 - \omega_g)\, h_1(j) / h_1^{max})$
      \For{$j \in Cand$}
        \If{$t = 1$}
          \State $o(j) = 1$
        \Else
          \State $\{j_1, j_2\} = S_j$
          \State $o(j) = \dfrac{(x_{j_1} - x_j, x_{j_2} - x_j)}{\|x_{j_1} - x_j\| \|x_{j_2} - x_j\|}$
          \State $h(j) = -(\omega_o o(j) - (1-\omega_o) h(j))$
        \EndIf
      \EndFor

      \State Sort $Cand$ based on $h$ metric

      \For{$k \in \{~j \in Cand ~|~ h_2(j) \ge 2.6 \mbox{ and } o(j) > -0.2~\}$}
        % Same as in algorithm for pressure points
        \State $D_3 = \{ ~j ~|~ dist(V_k,V_j, E) \le 3~ \}$ \
        \State $D_4 = \{ ~j ~|~ dist(V_k,V_j, E) = 4~ \}$
        \State $S_j = S_j \cup k \hskip .2in \forall j \in D_3 $
        \State $D_3 = D_3 \setminus k$
        \State $C = C \cup k $
        \State $F = F \cup D_3$
        \State $[h_1, h_2] = \mbox{\func{update\_heuristics}}(V, E, S, x, k, h_1, h_2)$
      \EndFor
    \EndFor
  \end{algorithmic}
\end{algorithm}
